# Supplementary material for: All in One: Multi-Task Prompting for Graph Neural Networks (Extended Abstract)
Source: arXiv:2403.07040 source file (2024-03-11)
Supplement: Supplementary file 1 [file appendix.tex]

\appendix

\section{Appendix}\label{sec:app}
In this section, we supplement more experiments to evaluate the effectiveness of our framework further. 
% Here we first introduce additional datasets in section \ref{app:add_data}, then we evaluate the transferability on more datasets in section \ref{app:transfer}. We conduct multi-class classification tasks in section \ref{app:multi_class}, additional graph-level classification tasks in section \ref{app:gc}, regression tasks in section \ref{app:reg}, and link prediction tasks in section \ref{app:link}. 
% Section \ref{app:setting} introduces more detailed settings of our implementation
The source code is publicly available at \textcolor{cyan}{\url{https://anonymous.4open.science/r/mpg}}
%We open the source code at https://anonymous.4open.science/r/mpg.

\begin{table}[t]
\centering
\caption{Statistics of Additional Datasets}
\label{tab:data_graph_more}
\resizebox{0.48\textwidth}{!}{%
\begin{tabular}{@{}p{0.11\textwidth}<{\centering}|p{0.057\textwidth}<{\centering}|p{0.057\textwidth}<{\centering}|p{0.061\textwidth}<{\centering}|p{0.047\textwidth}<{\centering}|c@{}}
\toprule
Dataset        & \#Nodes & \#Edges & \#Features & \#Labels & \#Graphs \\ \midrule
ENZYMES        & 19,580   & 74,564   & 21         & 6      & 600       \\
ProteinsFull & 43,471   & 162,088  & 32         & 2        & 1,113      \\\midrule
Movielens   &10,352 & 100,836  & 100         & -       & 1       \\
QM9            & 2,333,625 & 4,823,498 & 16         & -     & 129,433    \\\midrule %19
% Synthie        & 38,000   & 138,342  & 15         & 4       & 400       \\
PersonalityCafe   &  100,340   & 3,788,032 &   100      &   0  &  1     \\
Facebook  & 4,039 &  88,234    &  1,283  &    0  &    1  \\
\bottomrule
\end{tabular}%
}
\end{table}
\begin{table}[t]
\centering
\caption{Multi-class node classification (100-shots)}
\label{tab:app_multiclass}
\resizebox{0.48\textwidth}{!}{%
\begin{tabular}{@{}c|cc|cc@{}}
\toprule
\multirow{2}{*}{Methods} & \multicolumn{2}{c|}{Cora} & \multicolumn{2}{c}{CiteSeer} \\
     & Acc (\%) & Macro F1 (\%) & Acc (\%)& Macro F1  (\%)     \\ \midrule
Supervised    & 74.11  & 73.26        & 77.33          & 77.64 \\\midrule
Pre-train and Fine-tune & 77.97      & 77.63        & 79.67     & 79.83 \\ \midrule
Prompt     & 80.12      & 79.75        &  80.50   & 80.65    \\
Prompt w/o h    & 78.55          & 78.18            & 80.00     & 80.05  \\ \midrule
\makecell[c]{Reported Acc of GPPT\\ (Label Ratio 50\%)}  & 77.16      & -            & 65.81       & -   \\ 
% \midrule
% \makecell[c]{appr. Label Ratio of our 100 shots}  & \multicolumn{2}{c|}{$\sim 25\% $}   & \multicolumn{2}{c}{$\sim 18\% $}  \\ 
\bottomrule
\end{tabular}%
}
\end{table}

% \subsection{Additional Datasets}\label{app:add_data}
\textbf{Additional Datasets} Besides the datasets mentioned in the main experiments of our paper, we here supplement more datasets in Table \ref{tab:data_graph_more} to further evaluate the effectiveness of our framework.
%As shown in Table \ref{tab:data_graph_more} can be accessed from PyG Datasets.
% \footnote{\url{https://pytorch-geometric.readthedocs.io/en/latest/modules/datasets.html}}.
Specifically, ENZYMES and ProteinsFull are two molecule/protein datasets that are used in our additional graph-level classification tasks. 
% % In our main experiments of the paper, the graph-level labels are constructed by the node labels. Here the labels of these two datasets are their inborn graph classes which are not related to nodes. We do this because we wish to further confirm the effectiveness of our framework on graph-level tasks.
Movielens and QM9 are used to evaluate the performance of our method on edge-level and graph-level regression, respectively. In particular, Movielens contains user's rating scores to the movies, each edge in which has a score value ranging from $0$ to $5$. 
% We first use metapath2vec to get node initial features by meta path ``User-Movie-User'' and obtain 100 dimension features for all nodes. We scale the scoring values within $[0,1]$, and leverage our method to predict the edge value. 
QM9 is a molecule graph dataset where each graph has 19 regression targets, which are treated as graph-level multi-output regression. PersonalityCafe and Facebook datasets are used to test the performance of link prediction, both of which are social networks where edges denote the following/quoting relations. 

\textbf{Multi-label v.s. Multi-class Classification} In the main experiments, we treat the classification task as a multi-label problem. 
% treat each class as a binary classification problem to construct meta-learning tasks. Then we calculate the averaged performance on multiple tasks so that all tasks can share the same project head. This setting is a widely adopted solution to multi-label classification, which means one sample may belong to multiple labels. In other situations, however, we might be interested in the multi-class classification where each sample only belongs to one of the classes. 
Here we present the experimental results under a multi-class setting. 
%In this case, the output dimension of each model is exactly the same as the number of classes. 
% To save space, we only present the results on Cora and CiteSeer, but the similar observations are also reflected on other datasets. 
As reported in Table \ref{tab:app_multiclass}, our prompt-based method still outperforms the rest methods. 
%In particular, prompt w/o h, as mentioned in section \ref{subsub:com}, also suppresses the rest baselines, which further confirms the superiority of our method.

\textbf{Additional Graph-level Classification} Here, we evaluate the graph-level classification performance where the graph label is not impacted by nodes' attributes. As shown in Table \ref{tab:app_graph_multiclass}, 
% we only feed 100 labeled graphs for each graph class on the ProtensFull dataset and ENZYMES is tested with 50-shot setting, from which we can find that 
our method is more effective in the multi-class graph classification, especially in the few-shot setting.

\textbf{Edge/Graph-level Regression} Beyond classification tasks, our method can also support to improve graph models on regression tasks. Here, we evaluate the regression performance of both graph-level (QM9) and edge-level (MovieLens) datasets by MAE (mean absolute error) and MSE (mean squared error). We only feed 100-shot edge induced graphs for the model and the results are shown in Table \ref{tab:app_reg}, from which we can observe that our prompt-based methods outperform traditional approaches.

\textbf{Link Prediction} Beyond edge classification, link prediction is also a widely studied problem in the graph learning area. Here, the edges are split into three parts: (1) 80\% of the edges are for message passing only. (2) 10\% of the rest edges as the supervision training set. and (3) the rest edges as the testing set. For each edge in the training set and the testing set, we treat these edges as positive samples and sample non-adjacent nodes as negative samples. We generate the edge-induced graph for these node pairs according to the first part edges. The graph label is assigned as positive if the node pairs have a positive edge and vice versa. To further evaluate our method's potential in the extremely limited setting, we only sample 100 positive edges from the training set to train our model. In the testing stage, each positive edge has 100 negative edges. We evaluate the performance by MRR (mean reciprocal rank), and Hit Ratio@ 1, 5, 10. Results from Table \ref{tab:link} demonstrate that the performance of our prompt-based method still keeps the best in most cases.

\begin{table}[t]
\centering
\caption{Additional graph-level classification.}%\vspace{-0.15in}
\label{tab:app_graph_multiclass}
\resizebox{0.48\textwidth}{!}{%
\begin{tabular}{@{}c|cc|cc@{}}
\toprule
\multirow{2}{*}{Methods}  & \multicolumn{2}{c|}{ProteinsFull (100 shots)} & \multicolumn{2}{c}{ENZYMES (50 shots)} \\
     & Acc (\%)  & Macro F1 (\%)   & Acc (\%)& Macro F1 (\%)      \\ \midrule
Supervised    &  66.64 &  65.03   &  31.33  & 30.25 \\%\midrule
Pre-train + Fine-tune & 66.50  &66.43    & 34.67   & 33.94  \\ %\midrule
Prompt     &70.50  & 70.17    & 35.00  & 34.92 \\
Prompt w/o h   & 68.50  & 68.50 &  36.67  &  34.05
\\ \bottomrule
\end{tabular}%
}
\end{table}

\begin{table}[t]
\centering
\caption{Graph/edge-level regression with few-shot settings.}%\vspace{-0.15in}
\label{tab:app_reg}
\resizebox{0.48\textwidth}{!}{%
\begin{tabular}{@{}c|cc|cc@{}}
\toprule
Tasks    & \multicolumn{2}{c|}{Graph Regression} & \multicolumn{2}{c}{Edge Regression} \\
Datasets & \multicolumn{2}{c|}{QM9 (100 shots)} & \multicolumn{2}{c}{MovieLens (100 shots)} \\
Methods     & MAE  & MSE  & MAE  & MSE     \\ \midrule
Supervised    & 0.3006  & 0.1327   &0.2285 & 0.0895   \\%\midrule
Pre-train + Fine-tune & 0.1539  & 0.0351  &0.2171  &0.0774  \\ %\midrule
Prompt     &0.1384  & 0.0295   & 0.1949 &  0.0620   \\
Prompt w/o h   & 0.1424  &0.0341   & 0.2120    & 0.0744      
\\ \bottomrule
\end{tabular}%
}
\end{table}

\begin{table}[h]
\centering
\caption{Evaluation on link prediction (100-shot settings)}%\vspace{-0.15in}
\label{tab:link}
\resizebox{0.48\textwidth}{!}{%
\begin{tabular}{@{}c|cccc|cccc@{}}
\toprule
Datasets & \multicolumn{4}{c|}{PersonalityCafe} & \multicolumn{4}{c}{Facebook} \\
Methods     & MRR  & Hit@1 & Hit@5 & Hit@10& MRR  & Hit@1 & Hit@5 & Hit@10     \\ \midrule
Supervised  &0.18 & 0.04&0.24 &0.56  & 0.13&0.06 &0.17 &0.35 \\\midrule
\makecell[c]{Pre-train \\+ Fine-tune}  & 0.13&0.05 &0.12 &0.34  &0.10 &0.02 & 0.16& 0.33\\ \midrule
Prompt   &0.20 &0.07 &0.32 & 0.60 &0.19 &0.10 &0.23 &0.39  \\
Prompt w/o h   & 0.20&0.06 &0.30 & 0.50 &0.15 &0.09 &0.15 &0.33\\\midrule
\makecell[c]{Label Ratio}  & \multicolumn{4}{c|}{\makecell[c]{$\sim 0.003\%$ (training) \\ $\sim 80\%$(message passing)}}   & \multicolumn{4}{c}{\makecell[c]{$\sim 0.1\%$ (training) \\ $\sim 80\%$(message passing)}}  
\\ \bottomrule
\end{tabular}%
}
\end{table}

% \subsection{Algorithms of Induced Graph Generation for Nodes and Edges}
% Here we present three auxiliary algorithm: 
% Algorithms of Induced Graph Generation for Nodes and Edges, and episodes construction.

% \subsection{Visulization of Prompt Graph}
% \sun{try as much as you can if you still have some time.}
% \sun{To Be finished before 30 Jan}

% \subsection{Implementation Details}\label{app:setting}
% We implement our method by PyTorch\footnote{\url{https://pytorch.org}} and PyG\footnote{\url{https://www.pyg.org}} with Python 3.10. Most of the experiments are conducted on Mac Mini 2020 with Apple M1 chip, 16 GM memory and MacOS Ventura 13.1. A demo project is open available at https://anonymous.4open.science/r/mpg. We also developed a more advanced python package based on the paper source code. Following the anonymity policy, this package will also be released after the acceptance.

% Please add the following required packages to your document preamble:
% \usepackage{booktabs}
% \usepackage{multirow}
% \usepackage{graphicx}
\begin{table*}[h]
\centering
\caption{Edge-level performance (\%) with 100-shot setting. IMP (\%): the average improvement of prompt over the rest.}%\vspace{-0.15in}
\label{tab:edge_level}
\resizebox{0.99\textwidth}{!}{%
\begin{tabular}{@{}p{0.07\textwidth}<{\centering}c|p{0.025\textwidth}<{\centering}p{0.025\textwidth}<{\centering}p{0.035\textwidth}<{\centering}|p{0.025\textwidth}<{\centering}p{0.025\textwidth}<{\centering}p{0.035\textwidth}<{\centering}|p{0.025\textwidth}<{\centering}p{0.025\textwidth}<{\centering}p{0.035\textwidth}<{\centering}|p{0.025\textwidth}<{\centering}p{0.025\textwidth}<{\centering}p{0.035\textwidth}<{\centering}|p{0.025\textwidth}<{\centering}p{0.025\textwidth}<{\centering}p{0.035\textwidth}<{\centering}@{}}
\toprule
\multirow{2}{*}{\makecell[c]{Training\\ schemes}}     & \multirow{2}{*}{Methods} & \multicolumn{3}{c|}{Cora}       & \multicolumn{3}{c|}{CiteSeer}    & \multicolumn{3}{c|}{Reddit}     & \multicolumn{3}{c|}{Amazon} & \multicolumn{3}{c}{Pubmed}  \\
                                      &                          & Acc & F1 & AUC & Acc & F1 & AUC & Acc & F1 & AUC & Acc & F1 & AUC & Acc & F1 & AUC \\ \midrule
\multirow{3}{*}{supervised}           
 & GAT                        & 84.30    & 83.35    & 85.43     & 68.63    & 82.79    & 89.98     & 93.50    & 93.03    & 94.48     & 85.00    & 82.67    & 88.78     & 80.05    & 77.07    & 79.26     \\
                                      & GCN                        & 83.85    & 84.90    & 85.90     & 66.67    & 81.01    & 89.62     & 83.50    & 84.51    & 91.43     & 89.00    & 89.81    & 98.85     & 79.00    & 77.73    & 80.19     \\
                                      & GT          & 85.95    & 86.01    & 87.25     & 69.70    & 83.03    & 82.46     & 95.50    & 94.52    & 96.89     & 94.00    & 93.62    & 99.34     & 74.50    & 65.77    & 85.19      
\\\midrule
\multirow{6}{*}{\makecell[c]{pre-train \\+\\  fine-tune}}  
& GraphCL+GAT                & 85.64    & 85.97    & 87.22     & 72.67    & 82.85    & 92.98     & 94.00    & 93.75    & 98.43     & 86.50    & 86.96    & 84.47     & 85.54    & 83.92    & 91.78     \\
                                      & GraphCL+GCN                & 86.36    & 85.82    & 86.39     & 70.67    & 81.82    & 90.00     & 94.00    & 93.94    & 97.04     & 86.50    & 84.92    & 98.41     & 80.00    & 78.05    & 85.21     \\
                                      & GraphCL+GT  & 85.79    & 86.27    & 87.51     & 86.01    & 85.38    & 88.58     & 96.67    & 95.38    & 97.65     & 96.50    & 97.42    & 98.12     & 85.50    & 87.11    & 81.68     \\
                                      & SimGRACE+GAT               & 86.85    & 86.80    & 88.12     & 85.33    & 85.26    & 90.04     & 95.50    & 95.54    & 97.11     & 87.50    & 86.34    & 88.65     & 80.01    & 81.03    & 86.89     \\
                                      & SimGRACE+GCN               & 85.62    & 85.38    & 87.83     & 89.33    & 86.34    & 95.10     & 88.00    & 87.88    & 94.49     & 98.45    & 97.57    & 98.29     & 80.50    & 82.58    & 91.22     \\
                                      & SimGRACE+GT & 86.35    & 87.03    & 88.47     & 86.00    & 89.52    & 90.42     & 97.50    & 95.54    & 96.92     & 96.50    & 96.45    & 99.09     & 81.00    & 79.57    & 85.69      
\\\midrule
\multirow{6}{*}{prompt}               
  & GraphCL+GAT                & 86.85    & 86.88    & 87.92     & 76.67    & 83.00    & 96.22     & 95.36    & 94.50    & 98.65     & 88.50    & 86.00    & 87.15     & 86.50    & 84.75    & 92.61     \\
                                      & GraphCL+GCN                & 86.87    & 86.80    & 87.79     & 76.67    & 82.37    & 93.54     & 95.50    & 95.52    & 97.75     & 86.96    & 85.63    & 98.66     & 81.50    & 78.61    & 86.11     \\
                                      & GraphCL+GT  & 87.02    & 86.90    & 87.97     & 86.67    & 88.00    & 91.10     & 97.03    & 95.94    & 98.62     & 98.50    & 98.48    & 98.53     & 86.50    & 87.78    & 82.21     \\
                                      & SimGRACE+GAT               & 87.37    & 87.33    & 88.37     & 91.33    & 92.30    & 95.18     & 95.72    & 96.69    & 97.64     & 95.50    & 95.38    & 98.89     & 80.50    & 82.03    & 87.86     \\
                                      & SimGRACE+GCN               & 86.85    & 86.80    & 88.67     & 93.47    & 97.69    & 97.08     & 88.00    & 88.12    & 95.10     & 98.50    & 98.52    & 98.55     & 81.00    & 83.76    & 91.41     \\
                                      & SimGRACE+GT & 87.30    & 87.24    & 88.74     & 95.33    & 96.52    & 94.46     & 98.00    & 98.02    & 99.38     & 98.50    & 98.52    & 99.10     & 82.50    & 80.45    & 87.61       
\\\midrule
\multicolumn{2}{c|}{IMP(\%)}                                        & 1.65     & 1.48     & 1.28      & 12.26    & 6.84     & 5.21      & 1.94     & 2.29     & 1.88      & 3.63	&3.44&	2.03  & 2.98     & 4.66     & 3.21   \\\bottomrule
\end{tabular}%
}%\vspace{-0.1in}
\end{table*}
% Please add the following required packages to your document preamble:
% \usepackage{booktabs}
% \usepackage{multirow}
% \usepackage{graphicx}
\begin{table*}[h]
\centering
\caption{Graph-level performance (\%) with 100-shot setting. IMP (\%): the average improvement of prompt over the rest.}%\vspace{-0.15in}
\label{tab:graph_level}
\resizebox{0.99\textwidth}{!}{%
\begin{tabular}{@{}p{0.07\textwidth}<{\centering}c|p{0.025\textwidth}<{\centering}p{0.025\textwidth}<{\centering}p{0.035\textwidth}<{\centering}|p{0.025\textwidth}<{\centering}p{0.025\textwidth}<{\centering}p{0.035\textwidth}<{\centering}|p{0.025\textwidth}<{\centering}p{0.025\textwidth}<{\centering}p{0.035\textwidth}<{\centering}|p{0.025\textwidth}<{\centering}p{0.025\textwidth}<{\centering}p{0.035\textwidth}<{\centering}|p{0.025\textwidth}<{\centering}p{0.025\textwidth}<{\centering}p{0.035\textwidth}<{\centering}@{}}
\toprule
\multirow{2}{*}{\makecell[c]{Training\\ schemes}}     & \multirow{2}{*}{Methods} & \multicolumn{3}{c|}{Cora}       & \multicolumn{3}{c|}{CiteSeer}    & \multicolumn{3}{c|}{Reddit}     & \multicolumn{3}{c|}{Amazon} & \multicolumn{3}{c}{Pubmed}  \\
                                      &                          & Acc & F1 & AUC & Acc & F1 & AUC & Acc & F1 & AUC & Acc & F1 & AUC & Acc & F1 & AUC \\ \midrule
\multirow{3}{*}{supervised}      
& GAT                        & 84.40    & 86.44    & 87.60     & 86.50    & 84.75    & 91.75     & 79.50    & 79.76    & 82.11     & 93.05    & 94.04    & 93.95     & 69.86    & 72.30    & 66.92     \\
                                                                             & GCN                        & 83.95    & 86.01    & 88.64     & 85.00    & 82.56    & 93.33     & 64.00    & 70.00    & 78.60     & 91.20    & 91.27    & 94.33     & 61.30    & 59.97    & 66.29     \\
                                                                             & GT          & 85.85    & 85.90    & 89.59     & 77.50    & 75.85    & 89.72     & 69.62    & 68.01    & 66.32     & 90.33    & 91.39    & 94.39     & 60.30    & 60.88    & 67.62 
\\\midrule
\multirow{6}{*}{\makecell[c]{pre-train  \\ + \\fine-tune}}     
 & GraphCL+GAT                & 85.50    & 85.54    & 89.31     & 83.00    & 85.47    & 92.13     & 72.03    & 72.82    & 83.23     & 92.15    & 92.18    & 94.78     & 85.50    & 85.50    & 86.33     \\
                                                                             & GraphCL+GCN                & 85.50    & 85.59    & 87.94     & 86.50    & 84.57    & 94.56     & 71.00    & 71.90    & 80.33     & 93.58    & 93.55    & 94.93     & 78.75    & 77.29    & 89.40     \\
                                                                             & GraphCL+GT  & 85.95    & 85.05    & 87.92     & 84.50    & 81.87    & 88.36     & 69.63    & 70.06    & 81.35     & 91.68    & 91.55    & 94.78     & 86.85    & 86.93    & 88.91     \\
                                                                             & SimGRACE+GAT               & 86.04    & 86.33    & 88.55     & 83.50    & 85.84    & 90.09     & 81.32    & 81.64    & 88.61     & 93.58    & 93.57    & 93.91     & 87.33    & 86.70    & 88.02     \\
                                                                             & SimGRACE+GCN               & 85.95    & 86.05    & 89.33     & 84.50    & 86.46    & 91.60     & 80.50    & 81.52    & 89.11     & 90.73    & 90.52    & 94.85     & 85.26    & 84.64    & 86.99     \\
                                                                             & SimGRACE+GT & 86.40    & 86.47    & 89.64     & 81.00    & 81.54    & 89.81     & 69.50    & 70.97    & 77.11     & 92.63    & 92.56    & 94.04     & 85.95    & 86.05    & 89.37     
 \\\midrule
\multirow{6}{*}{prompt}
& GraphCL+GAT                & 86.40    & 86.47    & 89.46     & 86.50    & 89.93    & 92.24     & 73.36    & 73.32    & 84.77     & 94.08    & 94.02    & 94.20     & 85.95    & 85.97    & 87.17     \\
                                                                             & GraphCL+GCN                & 85.95    & 86.01    & 88.95     & 87.00    & 85.87    & 95.35     & 72.50    & 72.91    & 81.37     & 94.05    & 94.05    & 94.98     & 84.60    & 84.43    & 88.96     \\
                                                                             & GraphCL+GT  & 86.05    & 85.17    & 88.93     & 85.50    & 85.28    & 88.60     & 72.63    & 70.97    & 82.39     & 92.63    & 92.64    & 94.82     & 87.03    & 86.96    & 89.10     \\
                                                                             & SimGRACE+GAT               & 86.67    & 86.36    & 89.51     & 87.50    & 88.37    & 91.47     & 82.62    & 83.33    & 89.41     & 93.35    & 94.66    & 94.61     & 87.75    & 87.69    & 88.88     \\
                                                                             & SimGRACE+GCN               & 86.85    & 86.90    & 89.95     & 85.00    & 85.85    & 91.95     & 81.00    & 82.24    & 89.43     & 93.95    & 92.06    & 93.89     & 85.50    & 85.54    & 87.30     \\
                                                                             & SimGRACE+GT & 86.85    & 86.87    & 89.75     & 87.50    & 86.63    & 90.85     & 76.50    & 80.82    & 86.84     & 94.05    & 94.06    & 94.96     & 86.40    & 86.50    & 89.74      
\\\midrule
\multicolumn{2}{c|}{IMP(\%)}                                                                               & 1.12     & 0.43     & 0.79      & 3.52     & 4.54     & 0.53      & 4.69     & 4.31     & 6.13      &1.72&	1.39&	0.14 & 10.66    & 10.77    & 9.16     \\
\bottomrule
\end{tabular}%
}
\end{table*}
